# Supplementary material for: Accurate Predictions of Electron Binding Energies of Dipole-Bound Anions via Quantum Monte Carlo Methods
Source: arXiv:1809.09771 source file (2018-09-26)
Supplement: Supplementary file 1 [file supplement.pdf]

# Supplemental Information: Accurate Predictions of Electron Binding Energies of Dipole-Bound Anions via Quantum Monte Carlo Methods


Hongxia Hao,[†] James Shee,[‡] Shiv Upadhyay,[¶] Can Ataca,[§] Kenneth D. Jordan,[¶] and Brenda M. Rubenstein[*,†]

† *Department of Chemistry, Brown University, Providence, RI 02912*

‡ *Department of Chemistry, Columbia University, New York, NY 10027*

¶*Department of Chemistry, University of Pittsburgh, Pittsburgh, PA 15260*

§ *Department of Physics, University of Maryland - Baltimore County, Baltimore, MD 21250*

E-mail: brenda_rubenstein@brown.edu

Phone: (603) 661-2160

# Methods

Computing binding energies via projector quantum Monte Carlo techniques, such as Diffusion Monte Carlo (DMC)[1] or Auxiliary Field Quantum Monte Carlo (AFQMC),[2] is a three step process: first, molecular geometries are optimized using traditional quantum chemical methods; next, trial wave functions, which provide the necessary constraints for sign or phase problem-free quantum Monte Carlo calculations,[2–4] are generated using variational Monte Carlo (VMC)[5,6] and/or conventional quantum chemistry methods; and lastly, projector quantum Monte Carlo calculations are performed. We describe each of these steps in more detail below.

## Geometry Optimization

The geometries of the neutral molecules were first optimized using the MP2 method[7] together with the aug-cc-pVDZ basis set[8,9] in Gaussian 09.[10–13]

## Trial Wave Function Generation

Hartree-Fock (HF) wave functions generated in Gaussian 09,[12] GAMESS,[14,15] and NWChem[16] were used as trial wave functions in the DMC and AFQMC calculations. Spin-restricted Hartree Fock (RHF) wave functions were used for the neutral species, whereas spin-unrestricted Hartree Fock (UHF) wave functions were used for all of the anions except for $C_3H_2$, which necessitated the use of a Restricted Open-Shell Hartree Fock (ROHF) wave function. In order to obtain stable dipole-bound anions, it is essential to use flexible basis sets with very diffuse basis functions. Here, we used the aug-cc-pVDZ basis set[8,9] augmented with a set of diffuse $s$ and $p$ functions, and in one case, also $d$ functions.[17] With the exception of $C_3H_2O_3$, these diffuse functions were centered on an atom at the positive end of the molecular dipole, i.e., on the S atom in SO, on the H atom in HCN, and on the most positive C atom in $CH_3CN$ and $C_3H_2$. The exponents of the supplemental $s$, $p$ and $d$ functions form an even-tempered

sequence, with the ratio between consecutive exponents being 3.2 and the smallest exponent being 2.2x$10^{-5}$ $a_0^{-2}$ for each angular momentum. Diffuse functions were added until electron binding energies were observed to converge at the Hartree Fock level of theory. A $6s6p$ set of supplemental diffuse functions was used for HCN and $C_3H_2O_3$, a $7s7p$ set was used for SO, $CH_3CN$, and $CH_2CHCN$, and a $7s7p7d$ set was used for $C_3H_2$. For $C_3H_2O_3$, the diffuse functions were located at a point on the molecule's twofold rotational symmetry axis, but outside of the molecular ring. The location of this point was determined by scanning the line 60 degrees from both carbon atoms for the location that maximized the electron affinity according to Hartree Fock calculations (see Figure 1).

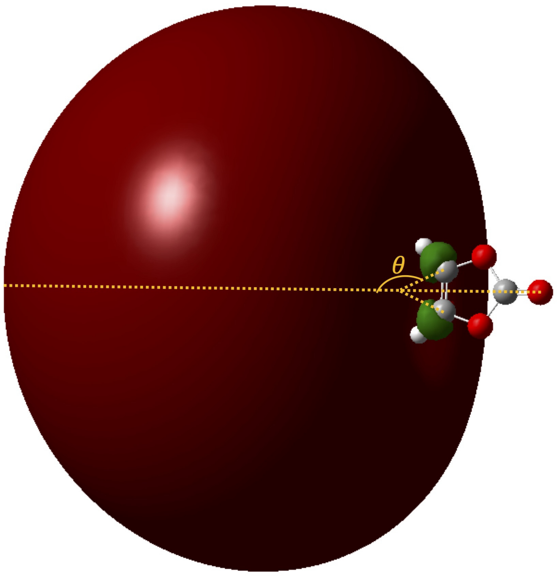


Figure 1: Visualization of the singly-occupied orbital of the $C_3H_2O_3$ anion as described by a UHF wave function. The isosurface value is taken as 0.003 e/Å$^3$.

## Diffusion Monte Carlo

DMC is a real-space projector quantum Monte Carlo method that has found great success in modeling a wide range of molecules and solids, and has therefore been extensively reviewed

in the literature.[1,6,18] Here, we summarize the algorithm for completeness. In DMC, a walker (sample) population representative of a trial wave function is propagated according to the imaginary time-dependent Schrödinger Equation

$$-\frac{\partial}{\partial\tau}\Psi(\vec{R},\tau) \quad = \quad \left(\hat{H}(\vec{R}) - E_T\right)\Psi(\vec{R},\tau) \tag{1}$$

where $\vec{R}$ denotes the real space coordinates of the system's electrons, $\tau$ denotes an imaginary time, $\Psi(\vec{R},\tau)$ denotes the time-dependent wave function, $\hat{H}(\vec{R})$ is the real space Hamiltonian, and $E_T$ is an arbitrary offset known as the reference energy. Solving this equation for large $\tau$ produces a distribution of walkers representative of the boson ground state wave function. In order to determine the fermion ground state wave function and to control the sign problem, an exponential decrease in the signal to noise ratio that develops in simulations of fermions as the projection time or number of walkers increases, the fixed-node approximation[3,19] must be employed. Equation (1) is first recast into an integral equation that makes it amenable to Monte Carlo sampling

$$f(\vec{R},\tau) = \int G(\vec{R} \leftarrow \vec{R}', \tau - \tau')f(\vec{R}',\tau')d\vec{R}'. \tag{2}$$

Here, $f(\vec{R},\tau) = \Psi_T(\vec{R})\Psi(\vec{R},\tau)$ is the product of a trial wave function $\Psi_T(\vec{R})$ and the sampled wave function, and $G(\vec{R} \leftarrow \vec{R}', \tau - \tau')$ is a Green's function describing the probability of moving from configuration $\vec{R}$ at time $\tau$ to a new configuration $\vec{R}'$ at time $\tau'$. In the short-time approximation, the Green's function may be broken into

$$\begin{aligned} & G(\vec{R} \leftarrow \vec{R}', \tau - \tau') \\ \approx \quad & \frac{1}{(2\pi\Delta\tau)^{3N/2}} e^{-\frac{[\vec{R}-\vec{R}'-\Delta\tau v(\vec{R}')]^2}{2\Delta\tau}} e^{-\frac{\Delta\tau}{2}[E_L(\vec{R})+E_L(\vec{R}')-2E_T]}, \end{aligned} \tag{3}$$

where $\Delta\tau \equiv \tau - \tau'$, $v(\vec{R}')$ is the drift velocity, and $E_L$ is the local energy. The first exponential is the drift-diffusion Green's function and the second exponential is the branching factor. In a typical DMC simulation, walkers sample the drift-diffusion Green's function for a new configuration and are then weighted by the branching term. In order to obtain a fermion ground state while preventing the walker weights from becoming negative, the fixed-node approximation is invoked which precludes walkers from crossing the nodal surface imposed by $\Psi_T$. Initial walker configurations are normally taken from Variational Monte Carlo (VMC) simulations.[6,18,20]

All VMC and DMC simulations in this work were performed using the CASINO package starting with the HF wave functions described above.[1] VMC calculations were performed to refine the HF trial wave functions in four sequential steps.[5] During the first step, the electron-electron ($U$) Jastrow parameters and cutoffs were optimized via variance minimization holding all electron-nuclear ($X$) terms constant. In the second step, the $X$ parameters and cutoffs were optimized holding the $U$ parameters and cutoffs optimized in the previous step constant. The electron-nuclear and electron-electron parameters were then optimized simultaneously using variance minimization. Lastly, during the fourth and final step, the linear (i.e., not cutoffs) electron-nucleus and electron-electron parameters were optimized using energy minimization. All VMC Jastrow optimizations were run for at least 240,000 time steps with 2,350 walkers. For the DMC simulations, averages were obtained by sampling the configurations of 4,650 walkers for 500,000 or more production steps, depending upon the magnitude of the error bars targeted. In order to obtain DMC energies in the $\Delta\tau \rightarrow 0$ limit, DMC simulations were conducted with three different time step sizes (see Tables 1 and 2 below for exact values) and then linearly extrapolated to yield the final values reported (see Figures 2 and 3). Charge density plots, shown in Figures 4 and 5, were constructed from samples taken from the smallest time step simulations of each species and visualized using the VESTA package.[21]

## Auxiliary Field Quantum Monte Carlo

Like DMC, AFQMC is a projector quantum Monte Carlo technique that applies a projection operator onto a trial wave function to obtain an approximation to the ground state wave function. What fundamentally distinguishes AFQMC from DMC is the fact that its imaginary time projection results in a random walk through a space of non-orthogonal Slater determinants.[2,22] Because of its reliance upon Slater determinants, AFQMC shares many commonalities with conventional quantum chemistry methods, such as configuration interaction and coupled cluster methods, in many ways making it easier to apply to chemical systems. In particular, AFQMC trial wave functions may readily be constructed from Hartree Fock and Multiconfigurational Self-Consistent Field wave functions and AFQMC makes use of the same one- and two-body integrals as produced by standard quantum chemistry software packages.[23–26] These benefits have made AFQMC an increasingly popular approach for modeling the electronic structure of a variety of atoms and molecules.[23–29] Because the details that underlie AFQMC have been presented elsewhere,[2,22] we will only review its key elements here.

Like DMC, AFQMC is predicated upon the projection equation

$$|\Psi_0\rangle \propto \lim_{n\to\infty} \left(e^{-\Delta\tau\hat{H}}\right)^n |\Psi_T\rangle, \tag{4}$$

where $|\Psi_0\rangle$ denotes the ground state wave function, $\Delta\tau$ is an increment of imaginary time, $\hat{H}$ is the system's many-body Hamiltonian, $|\Psi_T\rangle$ is the trial wave function, typically composed of one or more determinants, and $n$ is the number of times the projection operator is applied. In AFQMC, the *ab initio* Hamiltonian is written in second-quantized form as

$$\hat{H} = \hat{V} + \hat{K} = \frac{1}{2}\sum_{ijkl} V_{ijkl}\hat{c}_i^\dagger \hat{c}_j^\dagger \hat{c}_l \hat{c}_k + \sum_{ij} T_{ij}\hat{c}_i^\dagger \hat{c}_j. \tag{5}$$

Here, $i$, $j$, $k$, and $l$ denote different spin orbitals in a specified one-particle basis. $V_{ijkl}$ denotes the two-body and $T_{ij}$ the one-body integrals in this basis. $\hat{c}_i^\dagger$ represents a creation

operator that creates an electron in spin orbital $i$; $\hat{c}_j$ represents an annihilation operator that annihilates an electron in spin orbital $j$.[30] For ease of notation below, we moreover let $\hat{V}$ represent the collection of all two-body operators and $\hat{K}$ represent the collection of all one-body operators. Assuming $\Delta\tau$ is small, the projection operator may be factored into

$$e^{-\Delta\tau\hat{H}} \approx e^{-\Delta\tau\hat{K}/2} e^{-\Delta\tau\hat{V}} e^{-\Delta\tau\hat{K}/2} \tag{6}$$

where the Suzuki-Trotter factorization has been employed.[31,32] According to Thouless's Theorem,[33] the action of an exponential of a one-body operator on a determinant results in another determinant, reducing the process of projecting a one-body operator onto the initial wave function into standard matrix multiplication. However, no such theorem applies to exponentials of two-body operators. As derived elsewhere, the *ab initio* Hamiltonian may always be rewritten as the sum of squares of one-body operators. In particular, the two-body matrix elements, $V_{ijkl}$, may be expressed in terms of Cholesky vectors as $V_{ijkl} = \sum_\alpha L^\alpha_{ik} L^\alpha_{jl}$.[34] If each one-body operator is expressed as $\hat{v}_\alpha \equiv i \sum_{ik} L^\alpha_{ik} \sum_\sigma \hat{c}^\dagger_{i\sigma}\hat{c}_{k\sigma}$, then $\hat{V} = -\frac{1}{2}\sum_\alpha \hat{v}^2_\alpha$. The fact that the two-body potential may be written in terms of the squares of one-body operators makes it amenable to a continuous Hubbard-Stratonovich (HS) transformation[2,22]

$$e^{\Delta\tau\hat{v}^2_\alpha/2} = \frac{1}{\sqrt{2\pi}} \int_{-\infty}^{\infty} d\phi_\alpha e^{-\phi^2_\alpha/2} e^{\phi_\alpha\sqrt{\Delta\tau}\hat{v}_\alpha}, \tag{7}$$

where $\phi_\alpha$ is a scalar quantity known as an auxiliary field corresponding to term $\alpha$. This transformation is realized by sampling the auxiliary field $\phi_\alpha$ from a Gaussian distribution and then using that field to construct the one-body operator $e^{\phi_\alpha\sqrt{\Delta\tau}\hat{v}_\alpha}$. Combining these transformations for all $\alpha$ and inserting into Equation (6) yields the final expression for the propagator

$$e^{-\Delta\tau\hat{H}} \approx e^{-\Delta\tau\hat{K}/2}\Big[\int_{-\infty}^{\infty} P(\vec{\phi})\hat{B}(\vec{\phi})d\vec{\phi}\Big] e^{-\Delta\tau\hat{K}/2}. \tag{8}$$

Here, $\vec{\phi}$ denotes the vector of all $\alpha$ auxiliary fields, $P(\vec{\phi})$ denotes the Gaussian probability of a given set of fields, and $\hat{B}(\vec{\phi})$ is a collection of one-body operators. In a typical AFQMC simulation, walkers are first initialized to a trial wave function. Then, randomly-sampled instances of $e^{-\Delta\tau\hat{H}}$ are constructed according to Equation (8) and iteratively applied to each walker's trial wave function to realize a random walk through Slater determinant space. Simulations proceed until the stochastic error bars on observables averaged across the ensemble of walkers are small enough to meet a desired target.

Because the $\hat{v}_\alpha$ are typically imaginary, the HS transformation results in complex operators, and by extension, complex walker weights.[35] Averaging observables over these complex weights typically results in a phase problem that makes recovering meaningful observable averages from the noise impossible in a fixed amount of computational time.[35] In order to mitigate the noise incurred during the simulations, we perform background subtraction,[36] in which we subtract $\langle \hat{v}_\alpha \rangle$, the expectation value of $\hat{v}_\alpha$ with respect to the trial wave function, from $\hat{v}_\alpha$. We also apply a force bias[2,36] which minimizes the fluctuations of our walker weights with respect to the selected auxiliary fields by subtracting $\bar{\phi}_\alpha = -\sqrt{\Delta\tau}[\bar{v}_\alpha - \langle \hat{v}_\alpha \rangle]$, where $\bar{v}_\alpha \equiv \frac{\langle \Psi_T | \hat{v}_\alpha | \Psi \rangle}{\langle \Psi_T | \Psi \rangle}$, from $\phi_\alpha$. Combining these modifications, the one-body operator in Equation 7 becomes $e^{(\phi_\alpha - \bar{\phi}_\alpha)\sqrt{\Delta\tau}(\hat{v}_\alpha - \langle \hat{v}_\alpha \rangle)}$. By reducing the overall magnitude of the exponent in the propagator, the force bias and background subtraction substantially reduce the phase problem. Nevertheless, AFQMC simulations of molecules also necessitate employing the phaseless approximation. In the phaseless approximation,[35] after each propagation step, walker weights are projected back onto the real axis by multiplying them by $\max\{0, \cos(\Delta\theta)\}$, where the phase angle is defined as $\Delta\theta = \Im\{\ln \frac{\langle \Psi_T | \Psi^{(\tau+1)} \rangle}{\langle \Psi_T | \Psi^{(\tau)} \rangle}\}$. Combined with background subtraction and importance sampling, the phaseless approximation has been demonstrated to yield chemically accurate results on a wide range of benchmarks.[23–27,37]

## Correlated Sampling Auxiliary Field Quantum Monte Carlo

Correlated sampling has long been used in Variational, Diffusion, and Green's Function Monte Carlo methods,[38–41] and has most recently been extended to AFQMC.[42] In all of these approaches, differences between two quantities normally computed separately using independently generated configurations are instead computed using the same set of configurations. For sufficiently similar systems, this can result in a systematic cancellation of errors, which markedly reduces the variance associated with measured observables. The calculation of vertical binding energies involves energy differences between two species with identical molecular geometries, and thus is an ideal chemical application for correlated sampling.

In the context of AFQMC, correlated sampling involves using the same set of auxiliary fields to propagate both the neutral and anionic species, while each species' respective trial wave function is utilized to independently implement the phaseless constraint. To preserve maximal correlation between the walkers of the two species, we do not employ any standard population control techniques. This eliminates another possible source of bias due to a finite walker population, and is feasible when sufficiently small statistical error bars can be achieved at short imaginary times.

In this work, auxiliary fields are correlated from the start of the simulations, and measurements are performed following the protocol detailed in Reference 42. In brief, a set of independent simulations are initialized, each with a unique random number seed, and after an initial equilibration period, the mean and standard error of the cumulative averages are computed among the simulations. Convergence is attained when this mean is visually observed to plateau, and when the statistical error falls below a target threshold. The $\Delta\tau \rightarrow 0$ limit is estimated via linear extrapolations using simulations performed at $\Delta\tau = 0.01$ a.u. and $\Delta\tau = 0.005$ a.u.

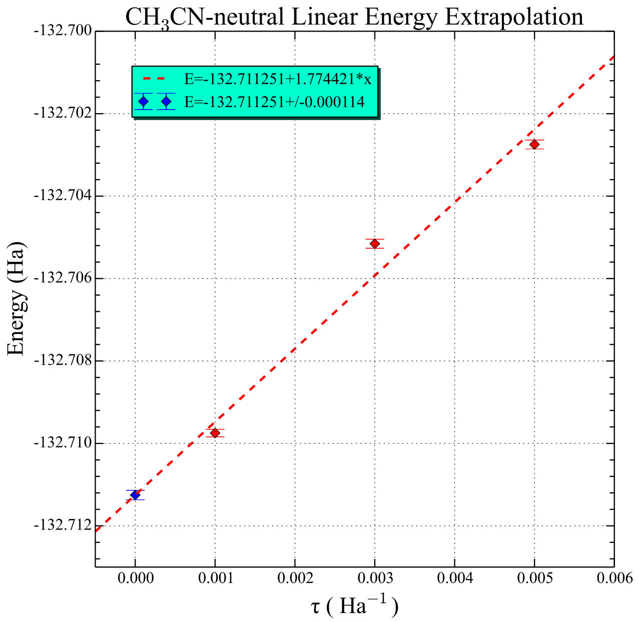


Figure 2: Extrapolation to zero time step of the DMC energy of $CH_3CN$. The calculations were preformed using an aug-cc-pvdz basis supplemented with diffuse $7s7p$ orbitals. RHF wave functions were provided as input into VMC calculations whose resulting Slater-Jastrow wave functions were employed as trial wave functions in the DMC calculations of the energies presented here.

# Diffusion Monte Carlo Time Step Extrapolations

**Table 1: DMC values of the ground state energies (Hartree) of the neutral species at different time steps sizes ($\text{Hartree}^{-1}$) used in the energy extrapolation.**

| | $\Delta\tau = 0.005$ | $\Delta\tau = 0.003$ | $\Delta\tau = 0.001$ |
|---|---|---|---|
| $CH_2CHCN$ | -170.761627+/-0.000099 | -170.764939+/-0.000090 | -170.770537+/-0.000192 |
| $CH_3CN$ | -132.702747+/-0.000107 | -132.705155+/-0.000110 | -132.709749+/-0.000092 |
| $C_3H_2$ | -115.272672+/-0.000187 | -115.275085+/-0.000178 | -115.278096+/-0.000169 |
| $C_3H_2O_3$ | -341.056016+/-0.000241 | -341.059574+/-0.000249 | -341.071200+/-0.000328 |
| | $\Delta\tau = 0.005$ | $\Delta\tau = 0.001$ | $\Delta\tau = 0.0007$ |
| HCN | -93.395107+/-0.000093 | -93.399181+/-0.000173 | -93.399520+/-0.000180 |
| | $\Delta\tau = 0.01$ | $\Delta\tau = 0.005$ | $\Delta\tau = 0.003$ |
| SO | -473.365793+/-0.000113 | -473.321900+/-0.000123 | -473.302764+/-0.000309 |

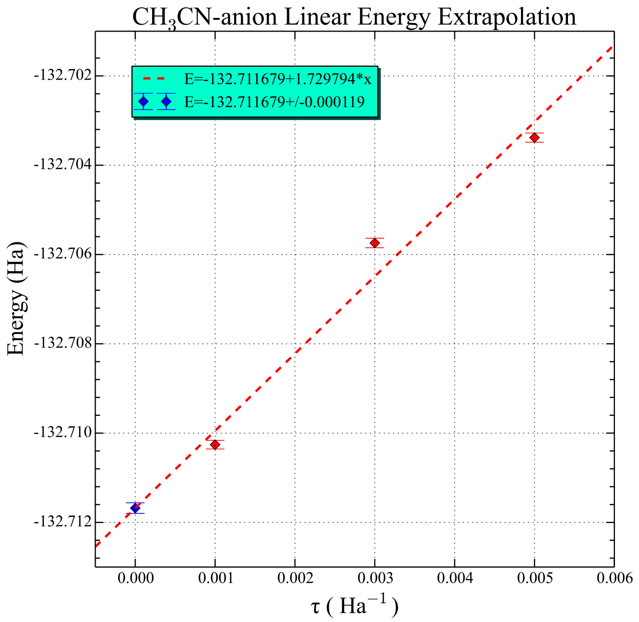


Figure 3: Extrapolation to zero time step of the DMC energy of $CH_3CN$ anion. The calculations were preformed using an aug-cc-pvdz basis supplemented with diffuse $7s7p$ orbitals. UHF wave functions were provided as input into VMC calculations whose resulting Slater-Jastrow wave functions were employed as trial wave functions in the DMC calculations of the energies presented here.

**Table 2: DMC values of the ground state energies (Hartree) of the anions (or neutral species plus an electron in the case of SO) at different time steps sizes (Hartree$^{-1}$) used in the energy extrapolation.**

| | $\Delta\tau = 0.005$ | $\Delta\tau = 0.003$ | $\Delta\tau = 0.001$ |
|---|---|---|---|
| $CH_2CHCN$ | -170.762150+/-0.000093 | -170.765430+/-0.000118 | -170.770631+/-0.000180 |
| $CH_3CN$ | -132.703381+/-0.000103 | -132.705742+/-0.000107 | -132.710259+/-0.000097 |
| $C_3H_2$ | -115.274067+/-0.000193 | -115.276134+/-0.000172 | -115.278942+/-0.000168 |
| $C_3H_2O_3$ | -341.057406+/-0.000248 | -341.061047+/-0.000267 | -341.071938+/-0.000332 |
| | $\Delta\tau = 0.005$ | $\Delta\tau = 0.001$ | $\Delta\tau = 0.0007$ |
| HCN | -93.395480+/-0.000084 | -93.399462+/-0.000144 | -93.399702+/-0.000188 |
| | $\Delta\tau = 0.01$ | $\Delta\tau = 0.005$ | $\Delta\tau = 0.003$ |
| SO | -473.373628+/-0.000093 | -473.325033+/-0.000119 | -473.304499+/-0.000287 |

# Charge Density Visualizations

Figures 4 and 5 report charge density plots from DMC calculations and visualized using VESTA.

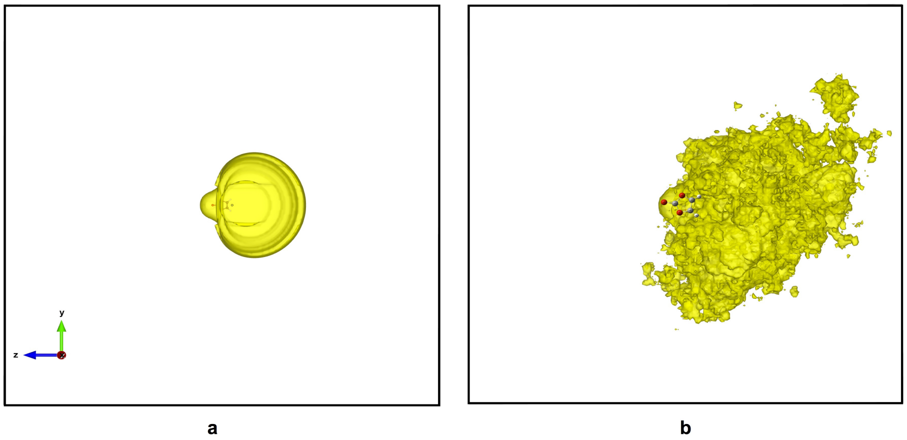


Figure 4: Charge density plots of the $C_3H_2O_3$ anion calculated using the (a) HF and (b) DMC methodologies. The isosurface value is taken as $3 \times 10^{-6}$ e/Å$^3$ for HF and $1 \times 10^{-13}$ e/Å$^3$ for DMC. Both methods showed a continuous and diffuse extra electron distribution.

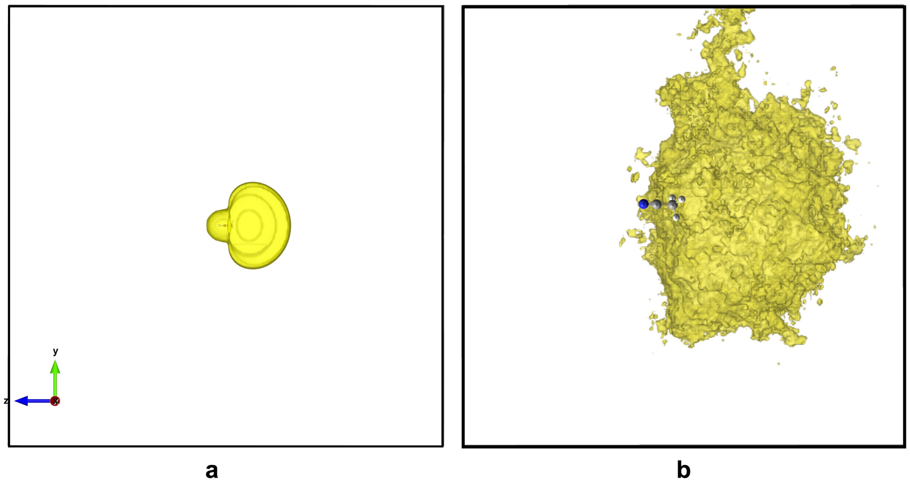


Figure 5: Charge density plots of the $CH_3CN$ anion calculated using the (a) UHF and (b) DMC methodologies. The isosurface value is taken as $3 \times 10^{-6}$ e/Å$^3$ for HF and $4 \times 10^{-14}$ e/Å$^3$ for DMC. Both methods showed a continuous and diffuse extra electron distribution.

## $C_3H_2$ Anion Trial Wave Functions

Our calculations on the $C_3H_2$ anion identified two different UHF solutions: one of which had sizable spin contamination, and the other of which, while displaying no spin contamination, had an unphysical charge distribution, with the charge density of the neutral core shifting in an unphysical manner in response to the excess electron. DMC calculations using the unphysical UHF trial wave function (i.e., that without spin contamination) encountered convergence issues. Using the same trial wave function, C-AFQMC calculations converged, but gave an EBE of $113.31 \pm 16.76$ $cm^1$, significantly smaller than the CCSD(T) value of 162 $cm^{-1}$. For this reason, the calculations reported in the main text were obtained using a spin-restricted HF trial function for the anion. These calculations gave a DMC EBE of $151.22 \pm 64.25$ $cm^{-1}$ and a C-AFQMC EBE of $132.45 \pm 9.43$ $cm^{-1}$, in closer agreement with the CCSD(T) value.

## References


(1) Foulkes, W. M. C.; Mitas, L.; Needs, R. J.; Rajagopal, G. Quantum Monte Carlo simulations of solids. *Rev. Mod. Phys.* **2001**, *73*, 33–83.

(2) Motta, M.; Zhang, S. Ab initio computations of molecular systems by the auxiliary-field quantum Monte Carlo method. *WIREs Comput. Mol. Sci. 8*, e1364.

(3) Ceperley, D. Fermion nodes. *J. Stat. Phys.* **1991**, *63*, 1237.

(4) Zhang, S.; Carlson, J.; Gubernatis, J. E. Constrained path Monte Carlo method for fermion ground states. *Phys. Rev. B* **1997**, *55*, 7464–7477.

(5) Drummond, N. D.; Needs, R. J. Variance-minimization scheme for optimizing Jastrow factors. *Phys. Rev. B* **2005**, *72*, 085124.

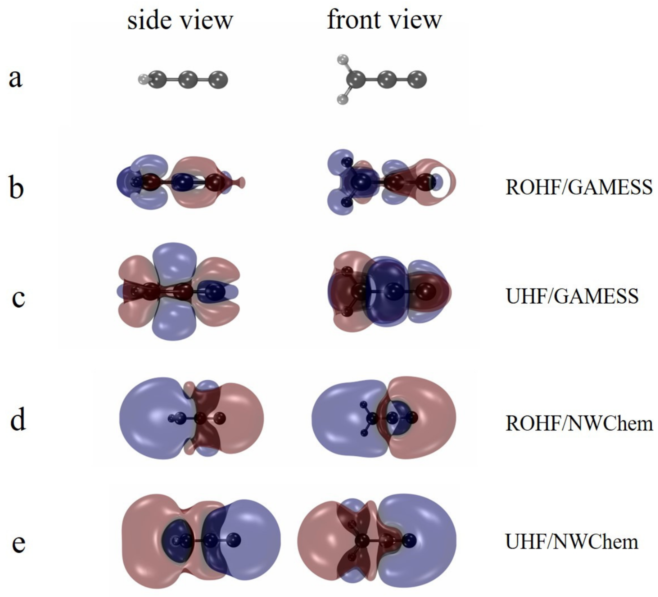


Figure 6: Change density differences between the $C_3H_2$ anion and the neutral excluding charge density representative of the excess electron from UHF and ROHF calculations performed in GAMESS and NWChem. Molecules in the left column are depicted from a side view; those in the right column are depicted from a front view. (a) Molecular geometries. Charge density differences between: (b) ROHF wave functions computed in GAMESS, (c) UHF wave functions computed in GAMESS, (d) ROHF wave functions computed in NWChem, and (e) UHF wave functions computed in NWChem. The isosurface value used in all cases is 0.0001 e/$\text{Å}^3$. Images are plotted using ORBKIT,[43] cclib,[44] and VMD.[45]

(6) Needs, R. J.; Towler, M. D.; Drummond, N. D.; Ríos, P. L. Continuum variational and diffusion quantum Monte Carlo calculations. *J. Phys.: Condens. Matter* **2010**, *22*, 023201.

(7) Møller, C.; Plesset, M. S. Note on an approximation treatment for many-electron systems. *Phys. Rev.* **1934**, *46*, 618–622.

(8) Dunning, T. H. Gaussian basis sets for use in correlated molecular calculations. I. The atoms boron through neon and hydrogen. *J. Chem. Phys.* **1989**, *90*, 1007–1023.

(9) Kendall, R. A.; Dunning, T. H.; Harrison, R. J. Electron affinities of the first-row atoms revisited. Systematic basis sets and wave functions. *J. Chem. Phys.* **1992**, *96*, 6796–6806.

(10) Frisch, M. J.; Head-Gordon, M.; Pople, J. A. A direct MP2 gradient method. *Chem. Phys. Lett.* **1990**, *166*, 275 – 280.

(11) Frisch, M. J.; Head-Gordon, M.; Pople, J. A. Semi-direct algorithms for the MP2 energy and gradient. *Chem. Phys. Lett.* **1990**, *166*, 281 – 289.

(12) Head-Gordon, M.; Pople, J. A.; Frisch, M. J. MP2 energy evaluation by direct methods. *Chem. Phys. Lett.* **1988**, *153*, 503 – 506.

(13) Saebo, S.; Almöf, J. Avoiding the integral storage bottleneck in LCAO calculations of electron correlation. *Chem. Phys. Lett.* **1989**, *154*, 83 – 89.

(14) Schmidt, M. W.; Baldridge, K. K.; Boatz, J. A.; Elbert, S. T.; Gordon, M. S.; Jensen, J. H.; Koseki, S.; Matsunaga, N.; Nguyen, K. A.; Su, S. et al. General atomic and molecular electronic structure system. *J. Comput. Chem.* *14*, 1347–1363.

(15) Gordon, M. S.; Schmidt, M. W. In *Theory and applications of computational chemistry*; Dykstra, C. E., Frenking, G., Kim, K. S., Scuseria, G. E., Eds.; Elsevier: Amsterdam, 2005; pp 1167 – 1189.

(16) Valiev, M.; Bylaska, E.; Govind, N.; Kowalski, K.; Straatsma, T.; Dam, H. V.; Wang, D.; Nieplocha, J.; Apra, E.; Windus, T. et al. NWChem: A comprehensive and scalable open-source solution for large scale molecular simulations. *Comput. Phys. Commun.* **2010**, *181*, 1477 – 1489.

(17) Gutowski, M.; Skurski, P.; Boldyrev, A. I.; Simons, J.; Jordan, K. D. Contribution of electron correlation to the stability of dipole-bound anionic states. *Phys. Rev. A* **1996**, *54*, 1906–1909.

(18) Toulouse, J.; Assaraf, R.; Umrigar, C. J. In *Electron correlation in molecules - ab initio beyond Gaussian quantum chemistry*; Hoggan, P. E., Ozdogan, T., Eds.; Advances in quantum chemistry; Academic Press, 2016; Vol. 73; pp 285 – 314.

(19) Anderson, J. B. A random-walk simulation of the Schrödinger equation: $H_3^+$. *J. Chem. Phys.* **1975**, *63*, 1499–1503.

(20) Rubenstein, B. In *Variational methods in molecular modeling*; Wu, J., Ed.; Molecular modeling and simulations (applications and perspectives); Springer, 2017.

(21) Momma, K.; Izumi, F. *VESTA3* for three-dimensional visualization of crystal, volumetric and morphology data. *J. Appl. Crystallogr.* **2011**, *44*, 1272–1276.

(22) Zhang, S. *Emergent phenomena in correlated matter: Modeling and simulation*; 2013; Vol. 3; Chapter Auxiliary-field quantum Monte Carlo for correlated electron systems.

(23) Al-Saidi, W. A.; Zhang, S.; Krakauer, H. Auxiliary-field quantum Monte Carlo calculations of molecular systems with a Gaussian basis. *J. Chem. Phys.* **2006**, *124*, 224101.

(24) Al-Saidi, W. A.; Krakauer, H.; Zhang, S. Auxiliary-field quantum Monte Carlo study of first- and second-row post-d elements. *J. Chem. Phys.* **2006**, *125*, 154110.

(25) Al-Saidi, W. A.; Krakauer, H.; Zhang, S. Auxiliary-field quantum Monte Carlo study of TiO and MnO molecules. *Phys. Rev. B* **2006**, *73*, 075103.

(26) Al-Saidi, W. A.; Krakauer, H.; Zhang, S. A study of H+$H_2$ and several H-bonded molecules by phaseless auxiliary-field quantum Monte Carlo with plane wave and Gaussian basis sets. *J. Chem. Phys.* **2007**, *126*, 194105.

(27) Suewattana, M.; Purwanto, W.; Zhang, S.; Krakauer, H.; Walter, E. J. Phaseless auxiliary-field quantum Monte Carlo calculations with plane waves and pseudopotentials: Applications to atoms and molecules. *Phys. Rev. B* **2007**, *75*, 245123.

(28) Purwanto, W.; Zhang, S.; Krakauer, H. An auxiliary-field quantum Monte Carlo study of the chromium dimer. *J. Chem. Phys.* **2015**, *142*, 064302.

(29) Josué Landinez Borda, E.; Gomez, J. A.; Morales, M. A. Non-orthogonal multi-slater determinant expansions in auxiliary field quantum Monte Carlo. *ArXiv e-prints* **2018**,

(30) Szabo, A.; Ostlund, N. *Modern quantum chemistry: Introduction to advanced electronic structure theory*; Dover Books on Chemistry; Dover Publications, 1989.

(31) Suzuki, M. Relationship between d-dimensional quantal spin systems and (d+1)-dimensional Ising systems - equivalence, critical exponents and systematic approximants of the partition function and spin correlations. *Prog. Theor. Phys.* **1976**, *56*, 1454–1469.

(32) Trotter, H. F. On the product of semi-groups of operators. *Proc. Am. Math. Soc.* **1959**, *10*, 545–551.

(33) Thouless, D. Stability conditions and nuclear rotations in the Hartree-Fock theory. *Nucl. Phys.* **1960**, *21*, 225 – 232.

(34) Purwanto, W.; Krakauer, H.; Virgus, Y.; Zhang, S. Assessing weak hydrogen binding on $Ca^+$ centers: an accurate many-body study with large basis sets. *J. Chem. Phys.* **2011**, *135*, 164105.

(35) Zhang, S.; Krakauer, H. Quantum Monte Carlo method using phase-free random walks with slater determinants. *Phys. Rev. Lett.* **2003**, *90*, 136401.

(36) Purwanto, W.; Zhang, S. Quantum Monte Carlo method for the ground state of many-boson systems. *Phys. Rev. E* **2004**, *70*, 056702.

(37) Purwanto, W.; Al-Saidi, W. A.; Krakauer, H.; Zhang, S. Eliminating spin contamination in auxiliary-field quantum Monte Carlo: realistic potential energy curve of $F_2$. *J. Chem. Phys.* **2008**, *128*, 114309.

(38) Filippi, C.; Umrigar, C. J. Correlated sampling in quantum Monte Carlo: A route to forces. *Phys. Rev. B* **2000**, *61*, R16291–R16294.

(39) Vrbik, J.; Legare, D. A.; Rothstein, S. M. Infinitesimal differential diffusion quantum Monte Carlo: Diatomic molecular properties. *J. Chem. Phys.* **1990**, *92*, 1221–1227.

(40) R., G. D. Extrapolation of the time-step bias in diffusion quantum Monte Carlo by a differential sampling technique. *J. Comput. Chem.* *10*, 176–185.

(41) Traynor, C.; Anderson, J. Parallel Monte Carlo calculations to determine energy differences among similar molecular structures. *Chem. Phys. Lett.* **1988**, *147*, 389 – 394.

(42) Shee, J.; Zhang, S.; Reichman, D. R.; Friesner, R. A. Chemical transformations approaching chemical accuracy via correlated sampling in auxiliary-field quantum Monte Carlo. *J. Chem. Theory Comput.* **2017**, *13*, 2667–2680.

(43) Hermann, G.; Pohl, V.; Tremblay, J. C.; Paulus, B.; Hege, H.-C.; Schild, A. ORBKIT: A modular python toolbox for cross-platform postprocessing of quantum chemical wavefunction data. *J. Comput. Chem.* *37*, 1511–1520.

(44) O'Boyle, N. M.; Tenderholt, A. L.; Langner, K. M. cclib: A library for package-independent computational chemistry algorithms. *J. Comput. Chem.* *29*, 839–845.

(45) Humphrey, W.; Dalke, A.; Schulten, K. VMD: Visual molecular dynamics. *J. Mol. Graphics* **1996**, *14*, 33 – 38.
